# Supplementary material for: Controlled Buckling and Crumpling of Nanoparticle-Coated Droplets
Source: arXiv:1011.4271 source file (2010-11-18)
Supplement: Supplementary file 1 [file dattashumweitz2010_supp.pdf]

Sujit S. Datta, Ho Cheung Shum, David A. Weitz

# SUPPORTING INFORMATION

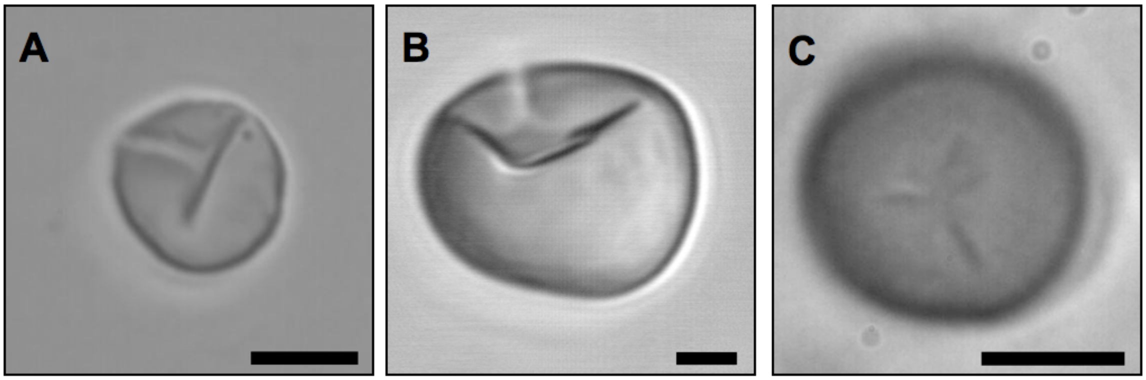


**Figure S1.** Optical micrographs of different buckled droplets, with multifaceted polyhedral indentations having three (A), four (B), and six (C) vertices. All scale bars are 5μm.

## Estimate of Two-Dimensional Shear Modulus of Droplet Surfaces

To understand the mechanical properties of the droplet interfaces, we directly measure the surface elastic shear modulus $G'_{2D}$ for a layer of nanoparticles at a flat fluid-fluid interface. Furthermore, we estimate $G'_{2D}$ by considering the microscopic interactions between adjacent nanoparticles. The measurement and theoretical estimate are in agreement with each other and suggest $G'_{2D} \approx$ 40-700mN/m.

We place an excess amount of nanoparticles at a flat interface between ethylene glycol and chlorobenzene and use an Anton-Paar Physica MCR501 rheometer equipped with an Interfacial Rheology System. We use a bicone geometry to directly measure the interfacial elastic and loss moduli $G'_{2D}$ and $G''_{2D}$ as a function of applied strain and frequency. The

results show that the layer of nanoparticles has mechanical properties similar to a soft glassy material (Ref. 13 in the main paper) with $G'_{2D} \approx 0.05$Pa.m = 50mN/m.

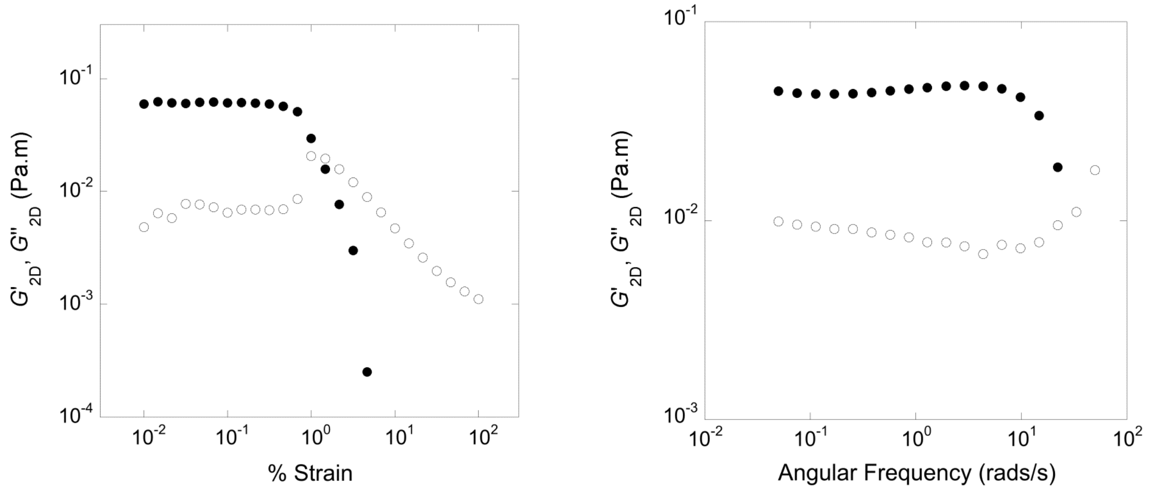


**Fig S2.** Interfacial shear and loss moduli $G'_{2D}$ (closed circles) and $G''_{2D}$ (open circles) as a function of applied strain at a fixed angular frequency of 5 rads/s (left image) and as a function of angular frequency at a fixed strain of 0.1% (right image).

To estimate $G'_{2D}$, we consider the energetics associated with interparticle interactions: namely, van der Waals interactions, attractive interactions due to their surface functionalization, and capillary interactions.

The van der Waals interaction can be estimated by $U_{vdW} = Aa_p/12l$, where $A$ is the Hamaker constant, $a_p$ is the nanoparticle radius, and $l$ is the distance between the nanoparticle surfaces[S1]. Using typical values of $A \approx 10^{-20}$ J and $l \approx 0.5$nm, we estimate $U_{vdW} \approx 3k_BT$ and hence, the two-dimensional shear modulus $G'_{2D} \approx U_{vdW}/a_p^2 \approx 0.2$mN/m.

The maximum value of the attractive interactions in the polar dispersed phase due to interpenetration of the alkyl chains coating the colloidal particles can be estimated by $U_{\mathrm{attr}} \approx \pi a_{\mathrm{p}} L^2 |1/2-\chi|/v_{\mathrm{m}}$ where $L$ is thickness of the surface coating layer, $\chi$ is the Flory-Huggins interaction parameter appropriate for the dispersed phase, and $v_{\mathrm{m}}$ is the volume of a solvent molecule (Ref. 25 in the main paper). Using suitable values of $L \approx 0.5$nm, $\chi \leq 10$, and $v_{\mathrm{m}} \approx 3$Å$^3$, we estimate a maximum value of $U_{\mathrm{att}} \approx 10^4 k_{\mathrm{B}}T$; thus, $G'_{\mathrm{2D}} \approx U_{\mathrm{att}}/a_{\mathrm{p}}^2 \approx$ 700mN/m.

By modeling a particle monolayer at a fluid interface interacting via capillary forces as an isotropic solid, Vella *et al.* (Ref. 6 in the main paper) and Arditty *et al.* (Ref. 8 in the main paper) independently developed an estimate for its Young's modulus: $E \sim 5\gamma/a_{\mathrm{p}}$, where $\gamma$ is the fluid-fluid interfacial tension and $a_{\mathrm{p}}$ is the particle radius. Using the interfacial tension for our system measured using pendant drop tensiometry ($\gamma \approx 7$mN/m), we use the expression for $E$ to estimate the energy of capillary interactions as $U_{\mathrm{cap}} \approx E a_{\mathrm{p}}^3 = 5\gamma a_{\mathrm{p}}^2 \approx 500 k_{\mathrm{B}}T$ and hence the two-dimensional shear modulus $G'_{\mathrm{2D}} \approx U_{\mathrm{cap}}/a_{\mathrm{p}}^2 \approx 40$mN/m.

These simple estimates suggest that the surface shear modulus at the droplet interfaces is likely to be determined predominantly by interparticle attractions due to their surface functionalization and capillary interactions, and is in the range $G'_{\mathrm{2D}} \approx 40\text{-}700$mN/m. This agrees with our measurement of $G'_{\mathrm{2D}} \approx 50$mN/m for a flat fluid-fluid interface saturated with an excess of nanoparticles. Nevertheless, additional detailed characterization of the

mechanical properties of Pickering emulsion droplet surfaces will provide further insights into the nature of the particle layer.

References

(S1) Israelachvili J. N. *Intermolecular and surface forces*; New York, 1992.
